# Supplementary material for: Quasi-1D Coulomb drag in the nonlinear regime
Source: arXiv:2410.17569 ancillary file (2025-07-24)
Supplement: Supplementary file 1 [file SM_Nonlinear_drag.pdf]

## Supplementary Materials: “Quasi 1D Coulomb drag in the nonlinear regime”

Mingyang Zheng,<sup>1</sup> Rebika Makaju,<sup>1</sup> Rasul Gazizulin,<sup>1,2</sup> Alex Levchenko,<sup>3</sup> Sathvikas J. Addamane,<sup>4</sup> and Dominique Laroche<sup>1,\*</sup>

<sup>1</sup>*Department of Physics, University of Florida, Gainesville, FL 32611, USA*

<sup>2</sup>*National High Magnetic Field Laboratory High B/T Facility,  
University of Florida, Gainesville, FL 32611, USA*

<sup>3</sup>*Department of Physics, University of Wisconsin–Madison, Madison, WI 53706, USA*

<sup>4</sup>*Center for Integrated Nanotechnologies, Sandia National Laboratories, Albuquerque, NM 87185, USA*

### DEVICE FABRICATION

The vertically-integrated double quantum wires used in this Letter are patterned on an n-doped GaAs/AlGaAs electron bilayer heterostructure (wafer VA1110). The two 18 nm wide quantum wells are separated by a 15 nm wide Al<sub>0.3</sub>Ga<sub>0.7</sub>As barrier. The unpatterned density and mobility of the GaAs quantum well are  $2.98 \times 10^{11} \text{ cm}^{-2}$ ,  $\mu = 7.4 \times 10^4 \text{ cm}^2/\text{V} \cdot \text{s}$ , respectively. Two sets of two split gates are deposited using electron beam lithography on the upper and the lower side of the sample using an epoxy-bound-and-stop-etch (EBASE) process. These gates define two wires that are  $\sim 5 \mu\text{m}$  long and  $\sim 0.6 \mu\text{m}$  wide. More details on the fabrication process are presented elsewhere [1]. A microscopy image of the finished vertically-integrated quantum wires is presented in Fig. S1(a), along with a zoom-in microscopy image of the wire overlapping region in Fig. S1(b). In Fig. S1(b), the lower wire design is overlapped with the zoom-in microscopy image, demonstrating the good alignment between the two quantum wires.

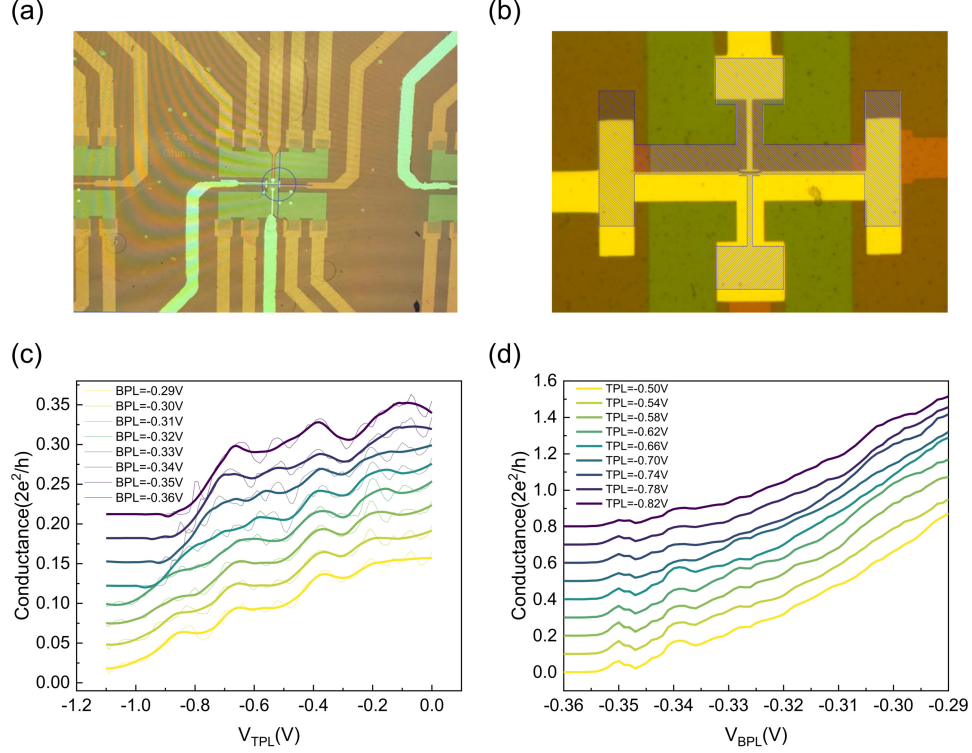

Fig. S1. Optical microscopy image and design of the vertical device. (a) Optical microscopy image of the vertical device. (b) Zoom-in image of the wire region. The wires overlapping region is shown. The lower wire design is overlapped with the zoom-in microscopy image. (c) Top (drive) wire conductance as a function of the top (drive) and bottom (drag) gate voltages. Interwire crosstalk is only visible on the lower end of the top wire gating range. Plateau-like features are clearly visible in the smoothed data (thick line). Successive line-cuts are vertically offset by 0.03 for visibility. (d) Bottom (drag) wire conductance as a function of bottom (drag) and Top (drive) gate voltages. Interwire crosstalk is negligible compared to the top(drive) wire. Successive line-cuts are vertically offset by 0.1 for visibility. The conductance plateaus are not quantized at integer values of  $2e^2/h$  as the wires are non-ballistic.

### ADDITIONAL DEVICE CHARACTERIZATION

A circuit diagram of the Coulomb drag measurement scheme utilizing a virtual ground on the drag side is presented in Fig. S2, where the drive current is applied on the top wire and the drag voltage is measured on the bottom wire. This setup ensures that no accidental bias is applied to the drag wire throughout the measurement. To prevent current flow from the drive wire to the drag wire, it is verified that tunneling between the two layers is negligible. The tunneling measurements are performed by sending a small source-drain voltage across the device for different top PO gate and bottom PO gate values, and then taking the numerical derivative of the resulting signal. Both top PO gate and bottom PO gate values were selected such that the tunneling resistance between the two wires was larger than  $10M\Omega$  in a bias range of  $\pm 1.5mV$ . Two examples of tunneling measurement are shown in Fig. S3. Fig. S3(a) and Fig. S3(b) show the tunneling conductance across the two layers when the top PO gate is at  $-0.39V$  and  $-0.43V$  respectively. The tunneling conductance is higher than  $10M\Omega$  when the top PO gate is at  $-0.43V$  and the bottom PO gate is below  $-0.36V$ .

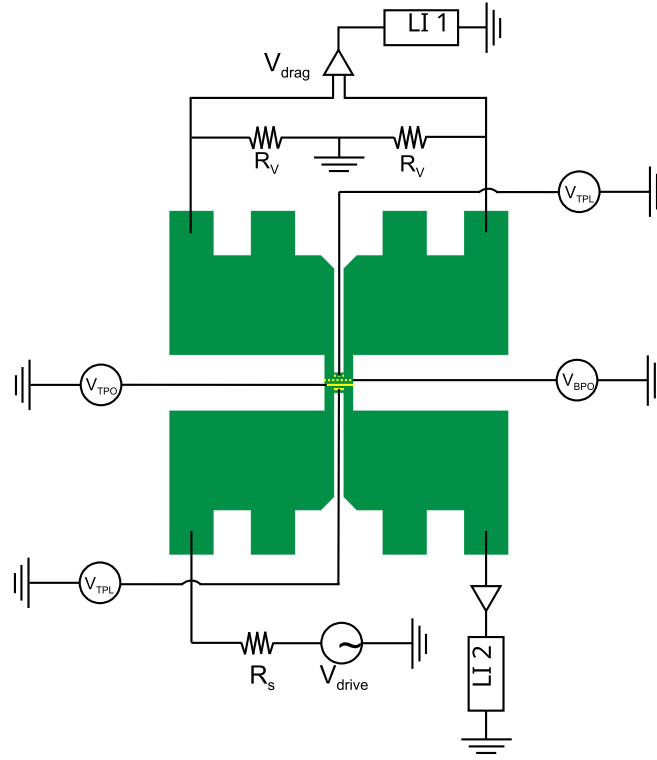

Fig. S2. Measurement setup. Circuit diagram for Coulomb drag measurements. A drive current is supplied to the top of the device and the drag voltage is measured in the bottom wire. The drive current is sourced using a  $R_s = 10\text{M}\Omega$  resistor in series with the drive wire. A virtual ground setup is used on the drag side of the experiment. Additionally, source-measure units are used to source and measure DC signals applied to the electrostatic gates.

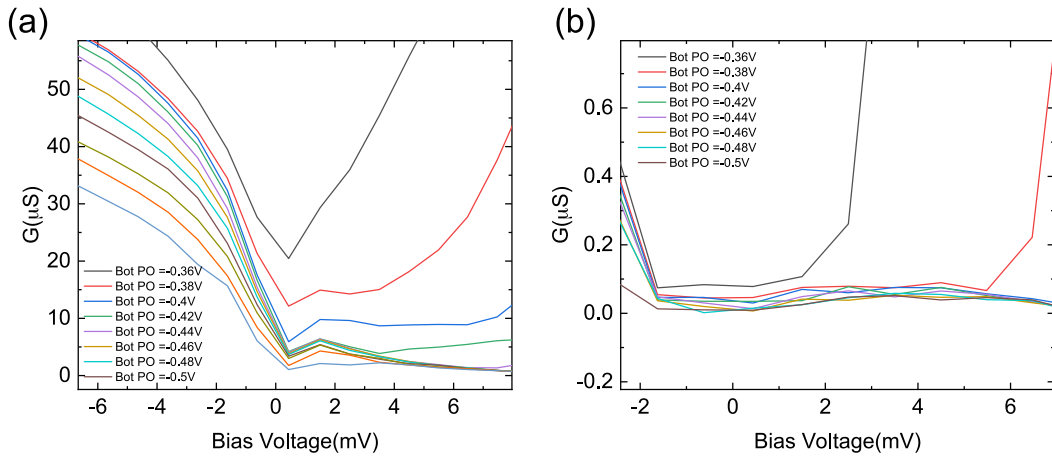

Fig. S3. Example of a 2D-2D tunneling measurement. The tunneling conductance is plotted against the source-drain bias across the tunnel barrier for various PO gate voltages. (a) The top PO gate at  $-0.39\text{V}$ , and (b) The top PO gate at  $-0.43\text{V}$ . The lines from top to bottom correspond to the bottom PO gate from  $-0.36\text{V}$  to  $-0.5\text{V}$  by  $-0.02\text{V}$  increments.

# DRIVE CURRENT DEPENDENT RECTIFIED DRAG

The momentum transfer and charge rectification components of rectified drag are shown in Fig. S4, as a function of the drag wire electron density and the drive current amplitude for two drive wire electron densities:  $N_{drive} = 2, TPL = -0.55V$  and  $N_{drive} = 1, TPL = -0.73V$ . For the momentum transfer component, as shown in Fig.S4(a) and Fig.S4(c), the amplitude of  $V_{drag}^{AS}$  increases significantly with decreasing drive wire electron density, and the signal is enhanced when both the drive and drag wires approach the first subband. That is consistent with the reduced screening effect and the density match enhanced Coulomb drag. Although the drag signal is strongly enhanced, the oscillation amplitude does not show a corresponding increase as the drive wire electron density decreases. For the charge rectification component, the nonlinearity and oscillations in the I-V relation are evident, with a strong nonmonotonous overall trend. Similar to the oscillations in  $V_{drag}^{AS}$  in the low drive current regime ( $I_{drive} < 20nA$ ),  $V_{drag}^S$  in the high current regime ( $I_{drive} > 20nA$ ) begins to decrease rapidly with increasing drive current and continues into the negative direction, as shown in Fig. S4(b) and Fig. S4(d), in stark contrast to the behavior of  $V_{drag}^{AS}$ . This behavior underscores the distinct physical mechanisms between the two components and warrants further investigation.

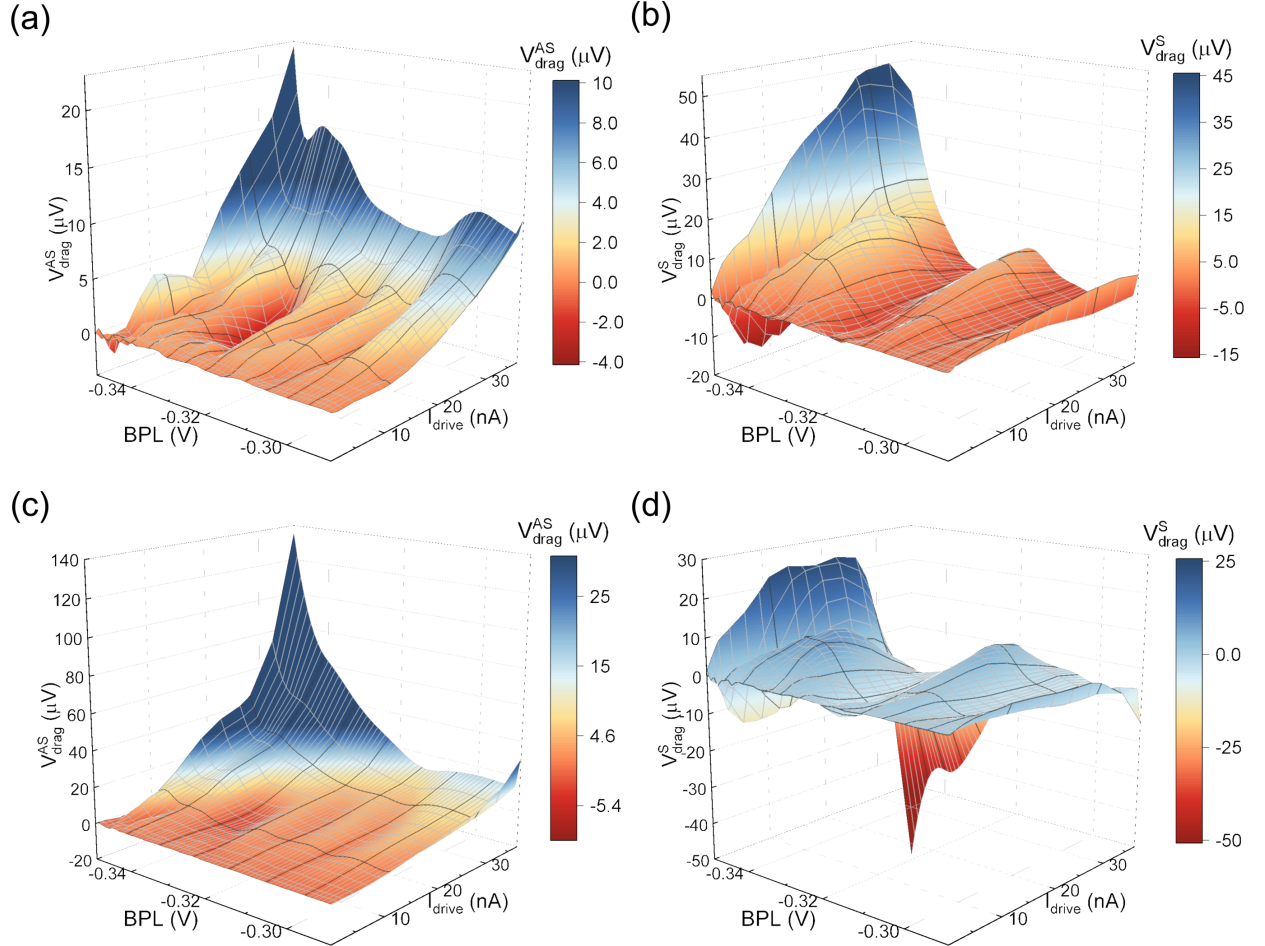

Fig. S4. Drive current dependent rectified drag. (a) Antisymmetric component  $V_{drag}^{AS}$ , (b) symmetric component  $V_{drag}^S$  of Coulomb drag as a function of the drag wire density and the drive current  $I_{drive}$  when the drive wire density is constant at  $TPL = -0.55V$  at base temperature. (c) Antisymmetric component  $V_{drag}^{AS}$ , (d) symmetric component  $V_{drag}^S$  of Coulomb drag as a function of the drag wire density and the drive current  $I_{drive}$  when the drive wire density is constant at  $TPL = -0.73V$  at base temperature.

# GATE AND DRIVE CURRENT TUNABLE RECTIFIED DRAG

The 2D maps of the symmetric component, antisymmetric component, and ratio  $r_{SAS}$  as a function of the top (drive) and the bottom (drag) gate voltages at different drive currents are shown in Fig. S5 at base temperature. For  $I_{drive} \simeq 0.85\text{nA}$ , both  $V_{drag}^S$  and  $V_{drag}^{AS}$  have similar amplitudes, with vertical stripes corresponding to the subband changing of the drag wire. As shown in Fig. S5(c), tunability is achieved by varying both drag wire and drive wire electron density, with the symmetric component dominating most regions. This dominance is further enhanced at a higher drive current of  $I_{drive} \simeq 4.6\text{nA}$ , as shown in Fig. S5(f). The increase in the drive current flattens some fine stripes in the drag maps and leads to a stronger increase in the  $V_{drag}^S$  from  $0.85\text{nA}$  to  $4.6\text{nA}$ . However, this dominance shifts when the drive current increases further. As shown in Fig. S5(j), the antisymmetric component becomes dominant in most regions, with only a few spots of symmetric component dominance. Additionally,  $V_{drag}^S$  changes sign to negative, with smeared-out subband stripes, while  $V_{drag}^{AS}$  remains positive throughout, showing a strong signal near the one subband region, consistent with Fig. S4. This negative  $V_{drag}^S$  rules out the heating effect as an explanation for the nonlinear I-V relation, as both components would be positive with smeared subbands at high temperatures ( $T > 1.5\text{K}$ ), as observed in previous work [2]. Therefore, this tunable contribution is achieved by adjusting both gate voltages and drive currents.

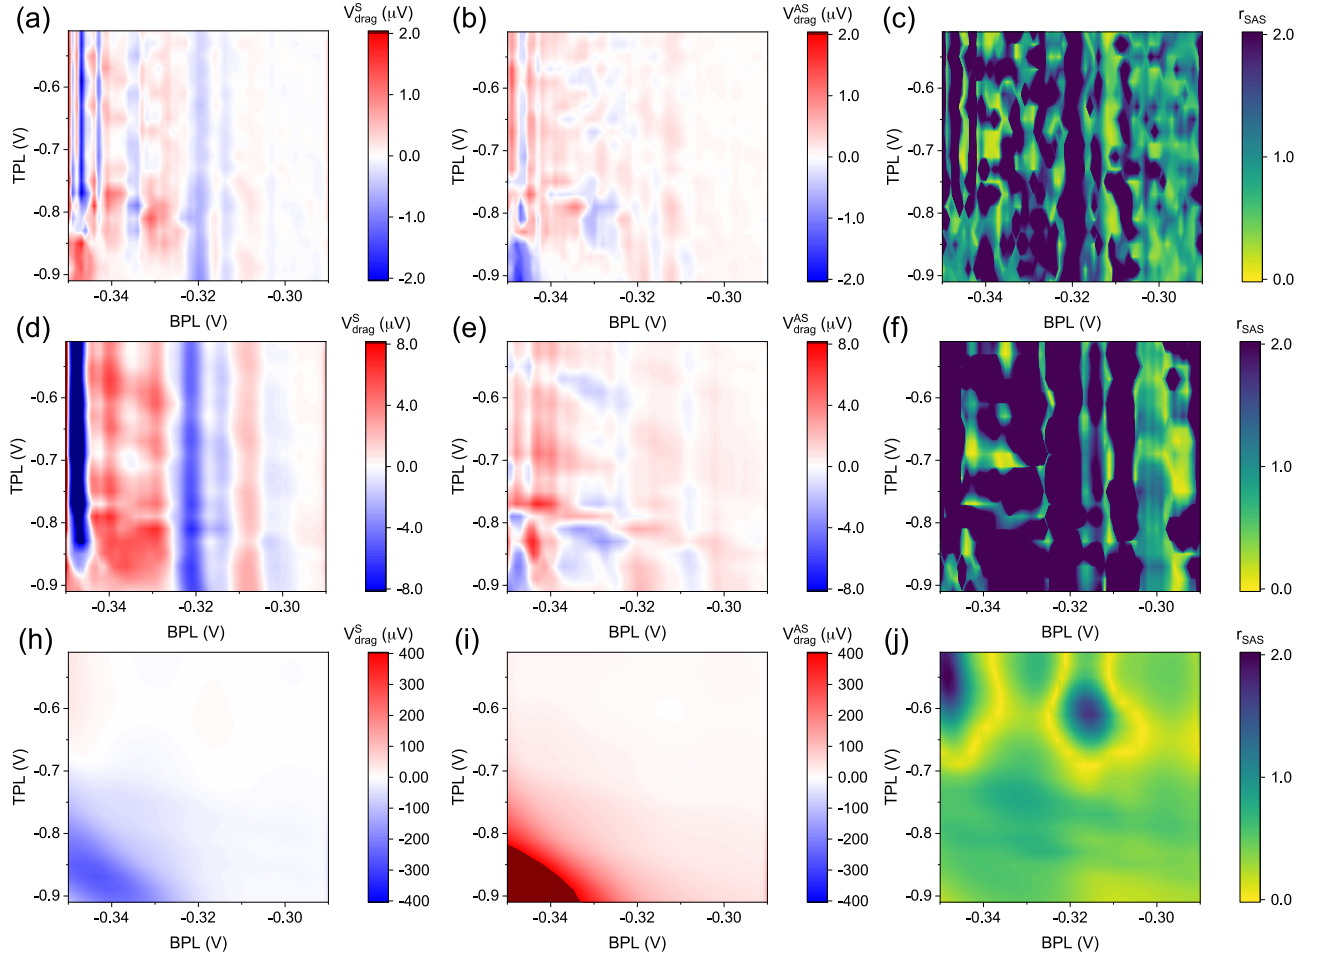

Fig. S5. Rectified drag ratio at base temperature. (a) Symmetric component  $V_{drag}^S$ , (b) antisymmetric component  $V_{drag}^{AS}$  and (c) ratio  $r_{SAS}$  of Coulomb drag as a function of the top (drive) wire density and the bottom (drag) gate voltages when the drive current is  $0.85\text{ nA}$ . (d), (e), (f) the  $V_{drag}^S$ ,  $V_{drag}^{AS}$  and  $r_{SAS}$  when the drive current is  $4.6\text{ nA}$ . (g), (h), (i) the  $V_{drag}^S$ ,  $V_{drag}^{AS}$  and  $r_{SAS}$  when the drive current is  $40\text{ nA}$ .

# MULTIMODE TOMONAGA-LUTTINGER LIQUID MODEL

In support of the analysis of the observed nonlinear Coulomb drag in our quantum wires, as presented in the main text, we consider a multimode generalization of the Tomonaga-Luttinger liquid model. The primary goal is to establish the functional form of the effective interaction parameters within each channel and their dependence on electron density, as well as the strength of interactions as different modes are populated.

The Hamiltonian of a wire consists of a free electron part and the electrostatic interaction (in units of  $\hbar = 1$ )

$$H = \sum_{l=1}^N \int \left( \frac{p_l^2}{2mn_l} + \frac{1}{2}mn_lv_l^2(\partial_x u_l)^2 \right) dx + \frac{1}{2} \sum_{ll'}^N \iint n_l n_{l'} (\partial_x u_l)(\partial_{x'} u_{l'}) V(x-x') dx dx' \quad (1)$$

Here  $n_l$  is the electron density in the  $l$ -th mode,  $u_l(x)$  is the displacement operator of electron liquid, and  $p_l(x)$  is the conjugate momentum density operator, so that the standard commutation relation holds  $[u_l(x), p_{l'}(x')] = i\delta_{ll'}\delta(x-x')$ , and velocity is proportional to the electron density  $v_l = \pi n_l/m$ , which is equal to the Fermi velocity in the noninteracting electron gas at this density. The form of the interaction term becomes transparent by realizing that the density perturbation  $\delta n$  is proportional to the deformation of the medium  $\delta n = -n\partial_x u$ . In the following we take the short-ranged interaction and substitute  $V(x-x') = V_0\delta(x-x')$ , where  $V_0$  is the zero-momentum Fourier component of the Coulomb potential. Assuming screening by a gate located at the distance  $d$  away from the quantum wire, we get with the logarithmic accuracy  $V_0 = \frac{2e^2}{\epsilon} \ln(k_F d)$ , where  $k_F$  is the Fermi wave vector of electrons in the wire,  $\epsilon$  is the dielectric constant of the host material.

With this simplification, the Hamiltonian in Eq. (1) becomes local and quadratic, and can be easily diagonalized by the orthogonal transformation

$$u_l(x) = \sqrt{\frac{2}{\pi n_l}} \sum_{l'}^N \Upsilon_{ll'} \int Q_{l'}(k) \sin(kx) dk, \quad (2)$$

$$p_l(x) = \sqrt{\frac{2n_l}{\pi}} \sum_{l'}^N \Upsilon_{ll'} \int P_{l'}(k) \sin(kx) dk \quad (3)$$

to a canonical form

$$H = \sum_l^N \int \left( \frac{1}{2m} P_l^2(k) + \frac{1}{2} m s_l^2 k^2 Q_l^2(k) \right) dk \quad (4)$$

In this representation the parameter  $s_l$  has the meaning of speed of plasmons for propagating density waves. To obtain this form of the Hamiltonian, the orthogonal matrix must satisfy the following eigenvalue equation

$$\sum_l^N (v_j^2 \delta_{jl} + \sqrt{v_j v_l} V_0 / \pi) \Upsilon_{lj'} = s_{j'}^2 \Upsilon_{jj'} \quad (5)$$

This equation can be explicitly resolved. Indeed, plasmon velocities can be found as roots of the following equation,

$$\sum_{l'}^N \frac{v_{l'}}{s_l^2 - v_{l'}^2} = \frac{\pi}{V_0} \quad (6)$$

whereas matrix elements are given by

$$\Upsilon_{ll'}^2 = \frac{v_l}{(s_l^2 - v_l^2)^2} \left[ \sum_j^N \frac{v_j}{(s_{l'}^2 - v_j^2)^2} \right]^{-1}. \quad (7)$$

The Luttinger interaction parameter for each eigenmode can be expressed as

$$g_l = (1 + \alpha_l) - \sqrt{(1 + \alpha_l)^2 - 1}, \quad (8)$$

where the auxiliary parameter

$$\alpha_l = \sum_{l'}^N \Upsilon_{ll'}^2 \frac{s_{l'}}{v_l} - 1 \quad (9)$$

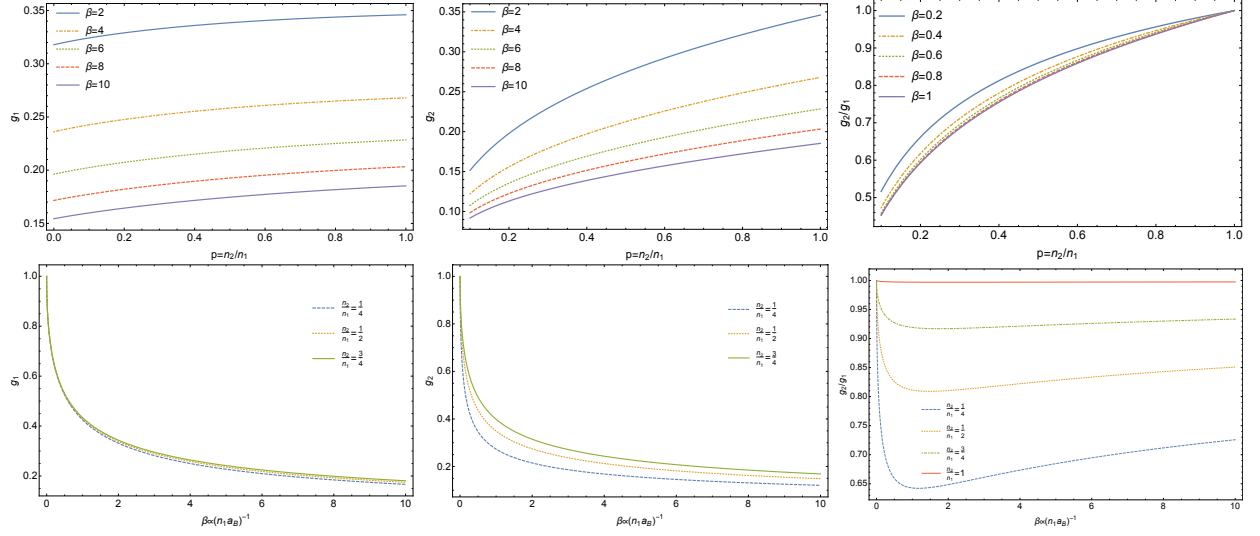

Fig. S6. The first row of figures shows  $g_1$ ,  $g_2$  and their ratio  $g_2/g_1$  as a function of density mismatch  $p = n_2/n_1$  plotted for several representative values of the dimensional interaction parameter corresponding to a moderately strong intrawire repulsion. The second row of figures shows the same results but plotted now as a function of interaction strength for different values of  $p$ .

is actually a power-exponent of the zero-bias anomaly in the density of states  $\nu_l(\varepsilon) \propto \varepsilon^{\alpha_l}$  [3–5].

In the closed form an explicit analytical solution can be found for the two-mode quantum wire. We normalize all plasmon velocities  $s_{1,2}$  in the units of the Fermi velocity in the first channel  $v_1$ . The solution of the quadratic equation for plasmon velocities gives

$$s_{1,2} = v_1 x_{1,2}, \quad x_{1,2}^2 = \frac{1}{2} \left[ (1 + p^2 + \beta(1 + p)) \pm \sqrt{(1 + p^2 + \beta(1 + p))^2 - 4(p^2 + \beta p(1 + p))} \right] \quad (10)$$

where we introduced  $p = n_2/n_1$  and dimensional parameter  $\beta = V_0/\pi v_1 = \frac{2}{\pi^2} \frac{\ln(k_F d)}{n_1 a_B}$ , with  $a_B = \epsilon/m e^2$  being the Bohr's radius. For the matrix elements we find

$$\Upsilon_{11}^2 = \frac{1}{(x_1^2 - 1)^2} \left[ \frac{1}{(x_1^2 - 1)^2} + \frac{p}{(x_1^2 - p^2)^2} \right]^{-1}, \quad (11)$$

$$\Upsilon_{12}^2 = \frac{1}{(x_2^2 - 1)^2} \left[ \frac{1}{(x_2^2 - 1)^2} + \frac{p}{(x_2^2 - p^2)^2} \right]^{-1}, \quad (12)$$

$$\Upsilon_{21}^2 = \frac{p}{(x_1^2 - p^2)^2} \left[ \frac{1}{(x_1^2 - 1)^2} + \frac{p}{(x_1^2 - p^2)^2} \right]^{-1}, \quad (13)$$

$$\Upsilon_{22}^2 = \frac{p}{(x_2^2 - p^2)^2} \left[ \frac{1}{(x_2^2 - 1)^2} + \frac{p}{(x_2^2 - p^2)^2} \right]^{-1}, \quad (14)$$

and for the auxiliary exponents

$$\alpha_1 = \Upsilon_{11}^2 x_1 + \Upsilon_{12}^2 x_2 - 1, \quad \alpha_2 = \Upsilon_{21}^2 \frac{x_1}{p} + \Upsilon_{22}^2 \frac{x_2}{p} - 1. \quad (15)$$

All these expressions ultimately define interaction parameters as a function of electron densities and bare strength of Coulomb interaction  $g_{1,2}(n_1, n_2, V_0)$ . In the limit of string repulsion  $\beta \gg 1$ , or equivalently  $V_0 \gg v_{1,2}$ , one can deduce an asymptotic result

$$g_1 \approx g_2 \approx \frac{\pi}{2} \sqrt{\frac{n a_B}{2 \ln(n d)}}, \quad (n a_B)^{-1} \gg 1 \quad (16)$$

with total density  $n = n_1 + n_2$  and plasmon velocity  $s \approx v_F/g_{1,2}$ . To explore the entire parameter space for arbitrary  $p = n_2/n_1$  and  $\beta$ , we plot  $g_{1,2}$  from explicit formulas of a two-channel model in Fig. S6.

---

\* **Email of Author to whom correspondence should be addressed:** dlaroc10@ufl.edu

- [1] D. Laroche, G. Gervais, M. P. Lilly, and J. L. Reno, Positive and negative Coulomb drag in vertically integrated one-dimensional quantum wires, *Nature Nanotechnology* **6**, 793 (2011).
- [2] M. Zheng, R. Makaju, R. Gazizulin, S. J. Addamane, and D. Laroche, Tunable contributions from rectification and momentum transfer to 1D Coulomb Drag (2024), arXiv:2408.12737 [cond-mat].
- [3] F. D. M. Haldane, Effective harmonic-fluid approach to low-energy properties of one-dimensional quantum fluids, *Phys. Rev. Lett.* **47**, 1840 (1981).
- [4] C. L. Kane and M. P. A. Fisher, Transport in a one-channel Luttinger liquid, *Phys. Rev. Lett.* **68**, 1220 (1992).
- [5] K. A. Matveev and L. I. Glazman, Coulomb blockade of tunneling into a quasi-one-dimensional wire, *Phys. Rev. Lett.* **70**, 990 (1993).
